# Supplementary material for: Distributional Individual Fairness in Clustering
Source: arXiv:2006.12589 source file (2020-06-22)
Supplement: Supplementary file 1 [file hardness.tex]

\section{NP-hardness of $k$-center with Individual Fairness}
\newcommand{\domset}{{\sc Dom-Set }}

In this section, we prove that the $k$-center problem with individual fairness constraints in NP-hard. Note that such a result does not follow trivially from the NP-hardness of vanilla $k$-center primarily because of two reasons. Firstly, the individually fair clustering is only required to output a distribution of assignments rather than a hard assignment of points to centers. Secondly, one needs to take care of the fairness constraints while doing the reduction. Indeed, as substantiated by out experiments, there could be instances where the optimal solution of a fair clustering is quite different from that of a vanilla clustering on the same instance. 

\begin{theorem}
The $k$-center problem with individual fairness   constraints is NP-hard.
\end{theorem}

We need the following lemma.
\begin{lemma}
\label{lem:fracToint}
Given a mapping from points in a metric space $(V,d)$ to distributions over $k$ centers with expected clustering distance over all points in $V$ to be $\rho$, there exists a solution to the corresponding vanilla k-center problem on $(V,d)$ of cost at the most $\rho$. 
\end{lemma}

\begin{proof}
Suppose for any point $v\in V$, $\mu_v$ be the distribution over the set of $k$ centers. Let $support(\mu_v)$ be the support of the distribution $\mu_v$. It is straightforward to see that assigning point $v\in V$ to the center $\cs_v = \text{argmin}_{c\in support(\mu_v)} d(c,v)$ forms a $k$-center clustering of cost at the most $\rho$.
\end{proof}

We reduce the well known dominating set problem (\domset) to $k$-center problem with individual fairness constraints  where the choice of the $f$-divergence function is $D_{\TV}$. In \domset, we are given an unweighted graph $G(v,E$ and a parameter $k$. The task is to decide whether there exists a subset $V'\subseteq V$ of size at the most $k$ such that for every $v\in V \setminus V'$, there exists an edge $(uv)\in E$ with $u\in V'$.

We require the following well-known theorem to complete our proof
\begin{theorem}[\cite{hopcroft2001introduction}]
\label{thm:dom-set hard}
\domset is NP-complete.
\end{theorem}

Now we are ready to prove the main theorem
\begin{proof}
Given any instance $G,k$ of \domset, we construct an instance of the $k$-center clustering as follows. The metric $d : V \times V \rightarrow \reals$ is defined as follows. $d(u, v) = 1$ if there exists $(uv)\in E$, otherwise $d(u, v) = 2$. 

Suppose we are given an individually fair $k$-center solution of expected cost $1$ to the above instance. Let $\calC = \{c_1, c_2, \cdots c_k\}$ be the set of open centers and $\mu_v$ be the distribution of any point $v$ on $\calC$. Since $d(v, c_i) \geq 1, \forall c_i\in \calC$, for any $c_i\in \calC$ such that $\mu_v(c_i) > 0$, $d(c_i, v) = 1$. Assigning $v$ to any such center certifies that the corresponding \domset instance $G,k$ has a solution.

Conversely, suppose the \domset instance $G,k$ admits a solution. We show that their exists a fair $k$-center solution with expected cost strictly less than $2$. It is a standard observation that the \domset solution can be converted to a $k$-center solution on the metric $d$ with cost 1, but not necessarily obeying the fairness constraints. We now prove that this solution can be modified to a fair solution which has expected cost {\em strictly less} than 2. Define $\calC$ to be the set of open centers in the possibly unfair solution. Pick an arbitrary center $\hatc\in \calC$. We define the distributions $\mu_v$ on $\calC$ for all points in $V$. For all $v\in V$, define $\mu_v(\hatc) = 0.5$ if and only if $v$ was not assigned to $\hatc$ in the $k$-center solution and $\mu_v(c') = 0.5$ if and only if $v$ was assigned to $c'$ in the $k$-center solution and $c' \neq \hatc$.   

We claim that the maximum expected distance of any point $v$ over the distribution $\mu_v$ is  strictly less than $2$. Let $c'\in calC$ be the center to which $v$ had been assigned in the $k$-center solution. Then, by definition of $\mu_v$, the expected distance of $v$ is $0.5d(v, \hatc) + 0.5d(v, c') < 2$ 

Now we show that the above distributions constitute a fair solution with respect to the statistical distance $D_{\TV}$. Consider any two points $v$ and $v'$. We recall the fact that since the distances between any two points in $d$ is either 1 or 2, $\bard(v, v') \geq 0.5$

There are a few cases as follows.
\bi
\item $v$ was assigned to $\hatc$ but $v'$ was assigned to $c'\neq \hatc$ : By construction of the distributions , $\mu_v(\hatc) = 1, \mu_{v'}(\hatc) = 0.5$ and $\mu_v(c') = 0, \mu_{v'}(c') = 0.5$. There are no other $c\in \calC$ in the support of either distributions. Hence, $D_{tv} (\mu_v, \mu_{v'}) = 0.5 \leq \bard(v,v')$ 

\item $v$ was assigned to $c$, $v'$ was assigned to $c'$ and $c\neq \hatc, c'\neq \hatc$ : Again, $\mu_v(\hatc) = \mu_{v'}(\hatc) = 0.5$, $\mu_v(c) = 0.5, \mu_{v'}(c) = 0$ and $\mu_v(c') = 0, \mu_{v'}(c') = 0$ and hence $D_{tv} (\mu_v, \mu_{v'}) = 0.5 \leq \bard(v,v')$

\item $v,v'$ were assigned to $\hatc$ : In this case, $D_{tv} = 0$ and the constraint is trivially satisfied.
\ei

Now assume their exists a polynomial time algorithm that optimally solves an individually fair $k$-center instance. Combining with Lemma~\ref{lem:fracToint}, this algorithm can then be used to distinguish between yes and no instances of \domset.

\end{proof}
